# Supplementary material for: Video-Text Representation Learning via Differentiable Weak Temporal Alignment
Source: arXiv:2203.16784 source file (2022-03-31)
Supplement: Supplementary file 2 [file supple_hard_negative.tex]

\begin{figure*}[t] 
    \centering
    \includegraphics[width=0.95\textwidth]{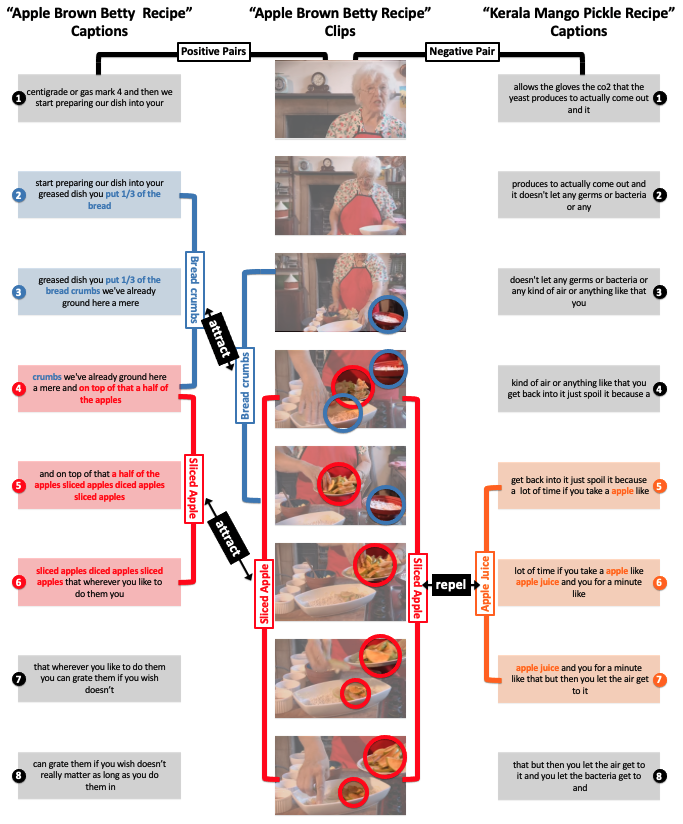}
    \vspace{-10pt}
    \caption{\textbf{Comparison between Positive Pairs and Hard Negative Pairs.} 
    The left captions and the right captions are positive pairs and negative pairs of the given center clips, respectively.
    The alignments between positive pairs are attracted each other and the alignments between negative pairs are repelled each other.
    }
    \label{fig:hard_negative}
    \vspace{5mm}
\end{figure*}
