# Supplementary material for: Video-Text Representation Learning via Differentiable Weak Temporal Alignment
Source: arXiv:2203.16784 source file (2022-03-31)
Supplement: Supplementary file 3 [file supple_hard_negative_path.tex]

\begin{figure}
    \centering
    \begin{subfigure}[b]{0.47\textwidth}  
        \centering 
        \includegraphics[width=\textwidth]{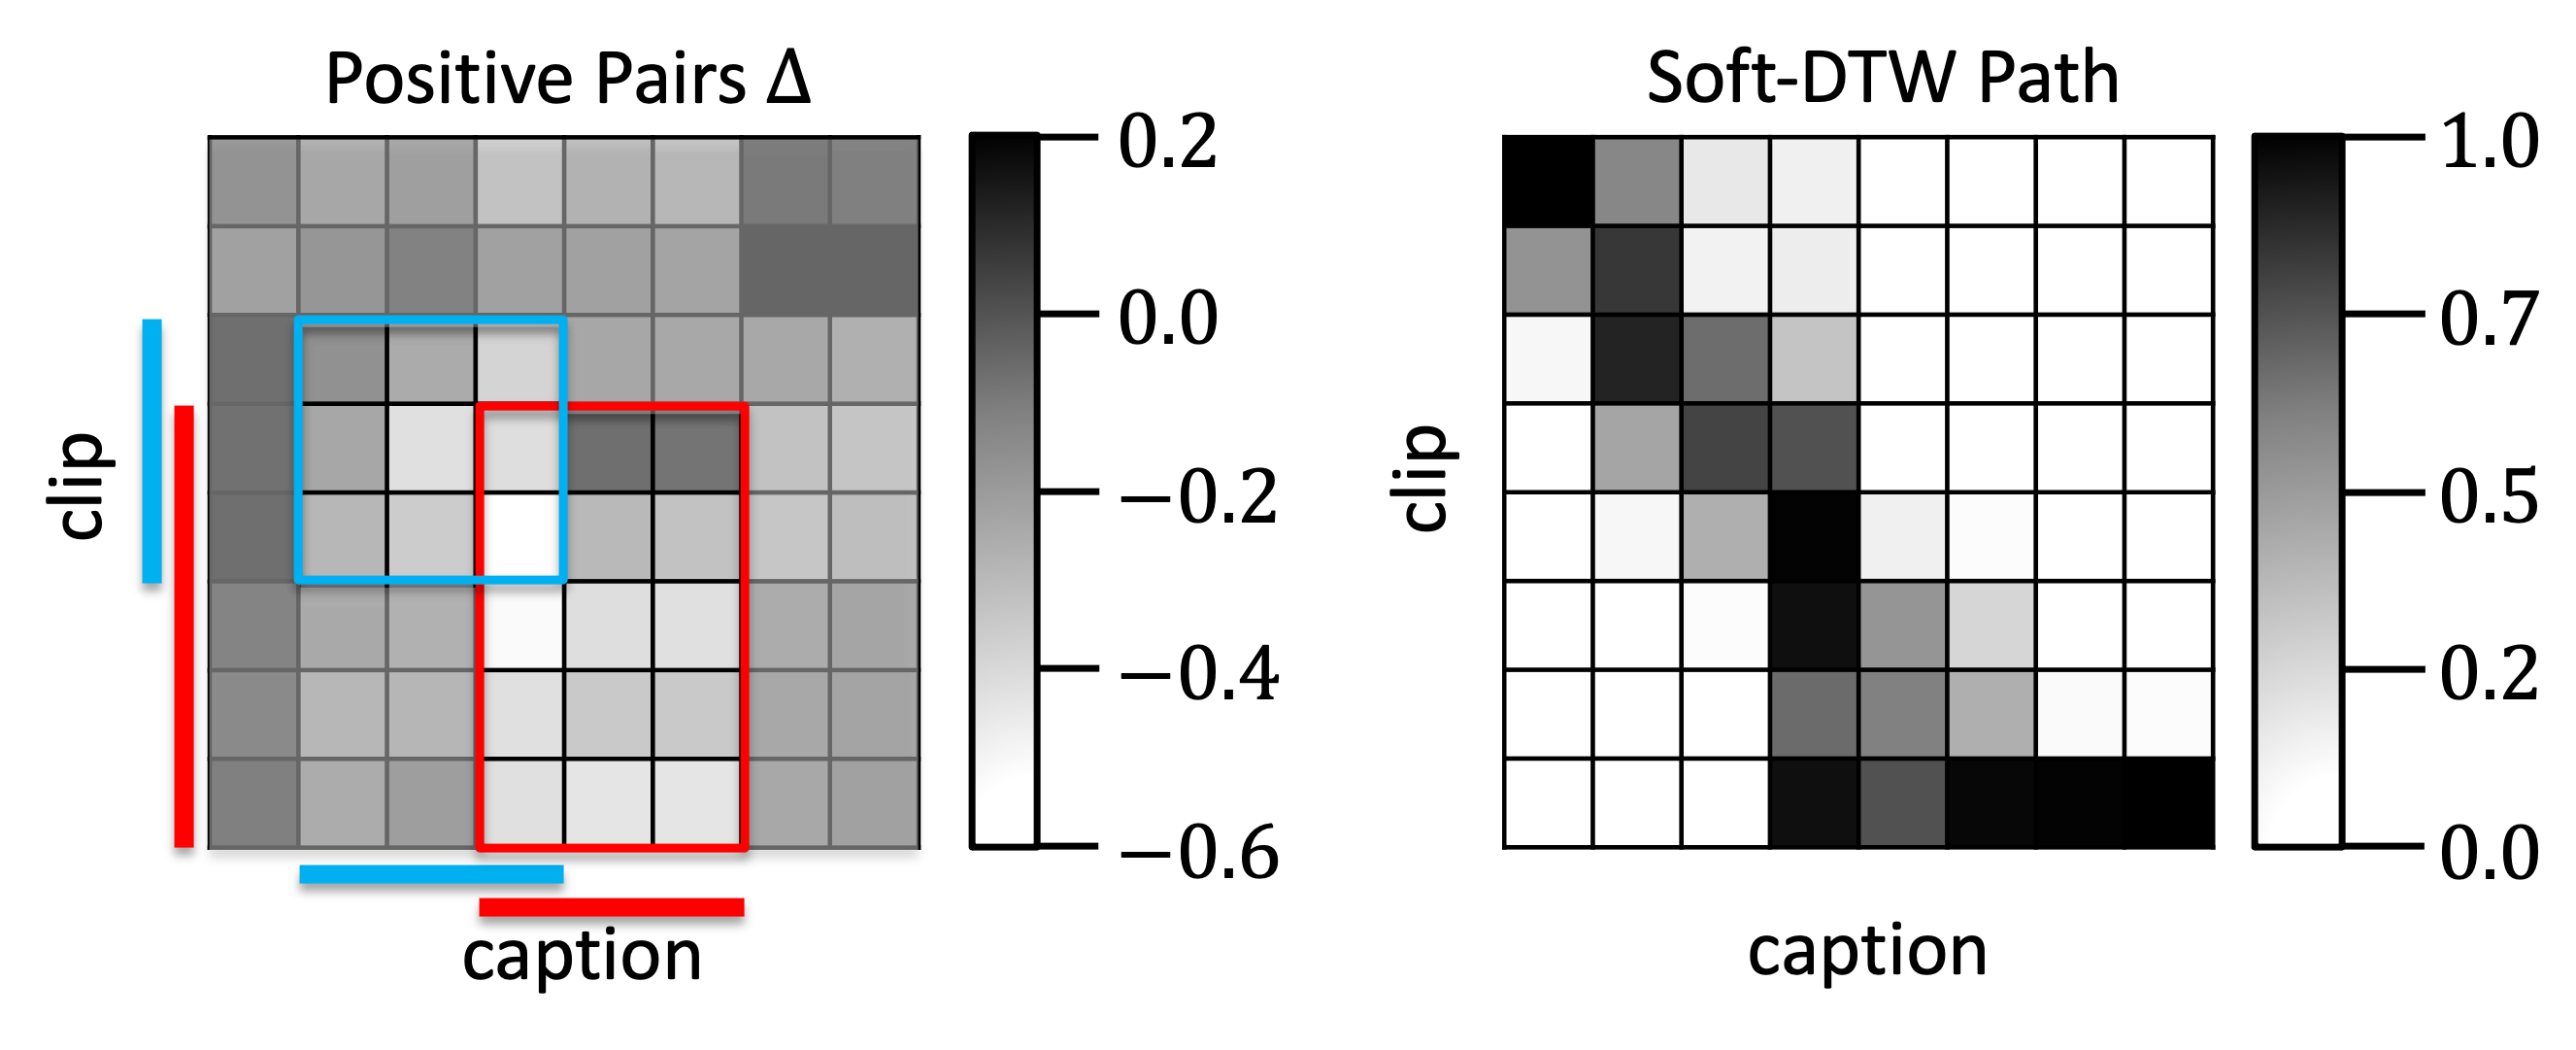}
        \caption{Positive Pairs.}
        \label{fig:positive}
    \end{subfigure}
    \begin{subfigure}[b]{0.47\textwidth}   
        \centering 
        \includegraphics[width=\textwidth]{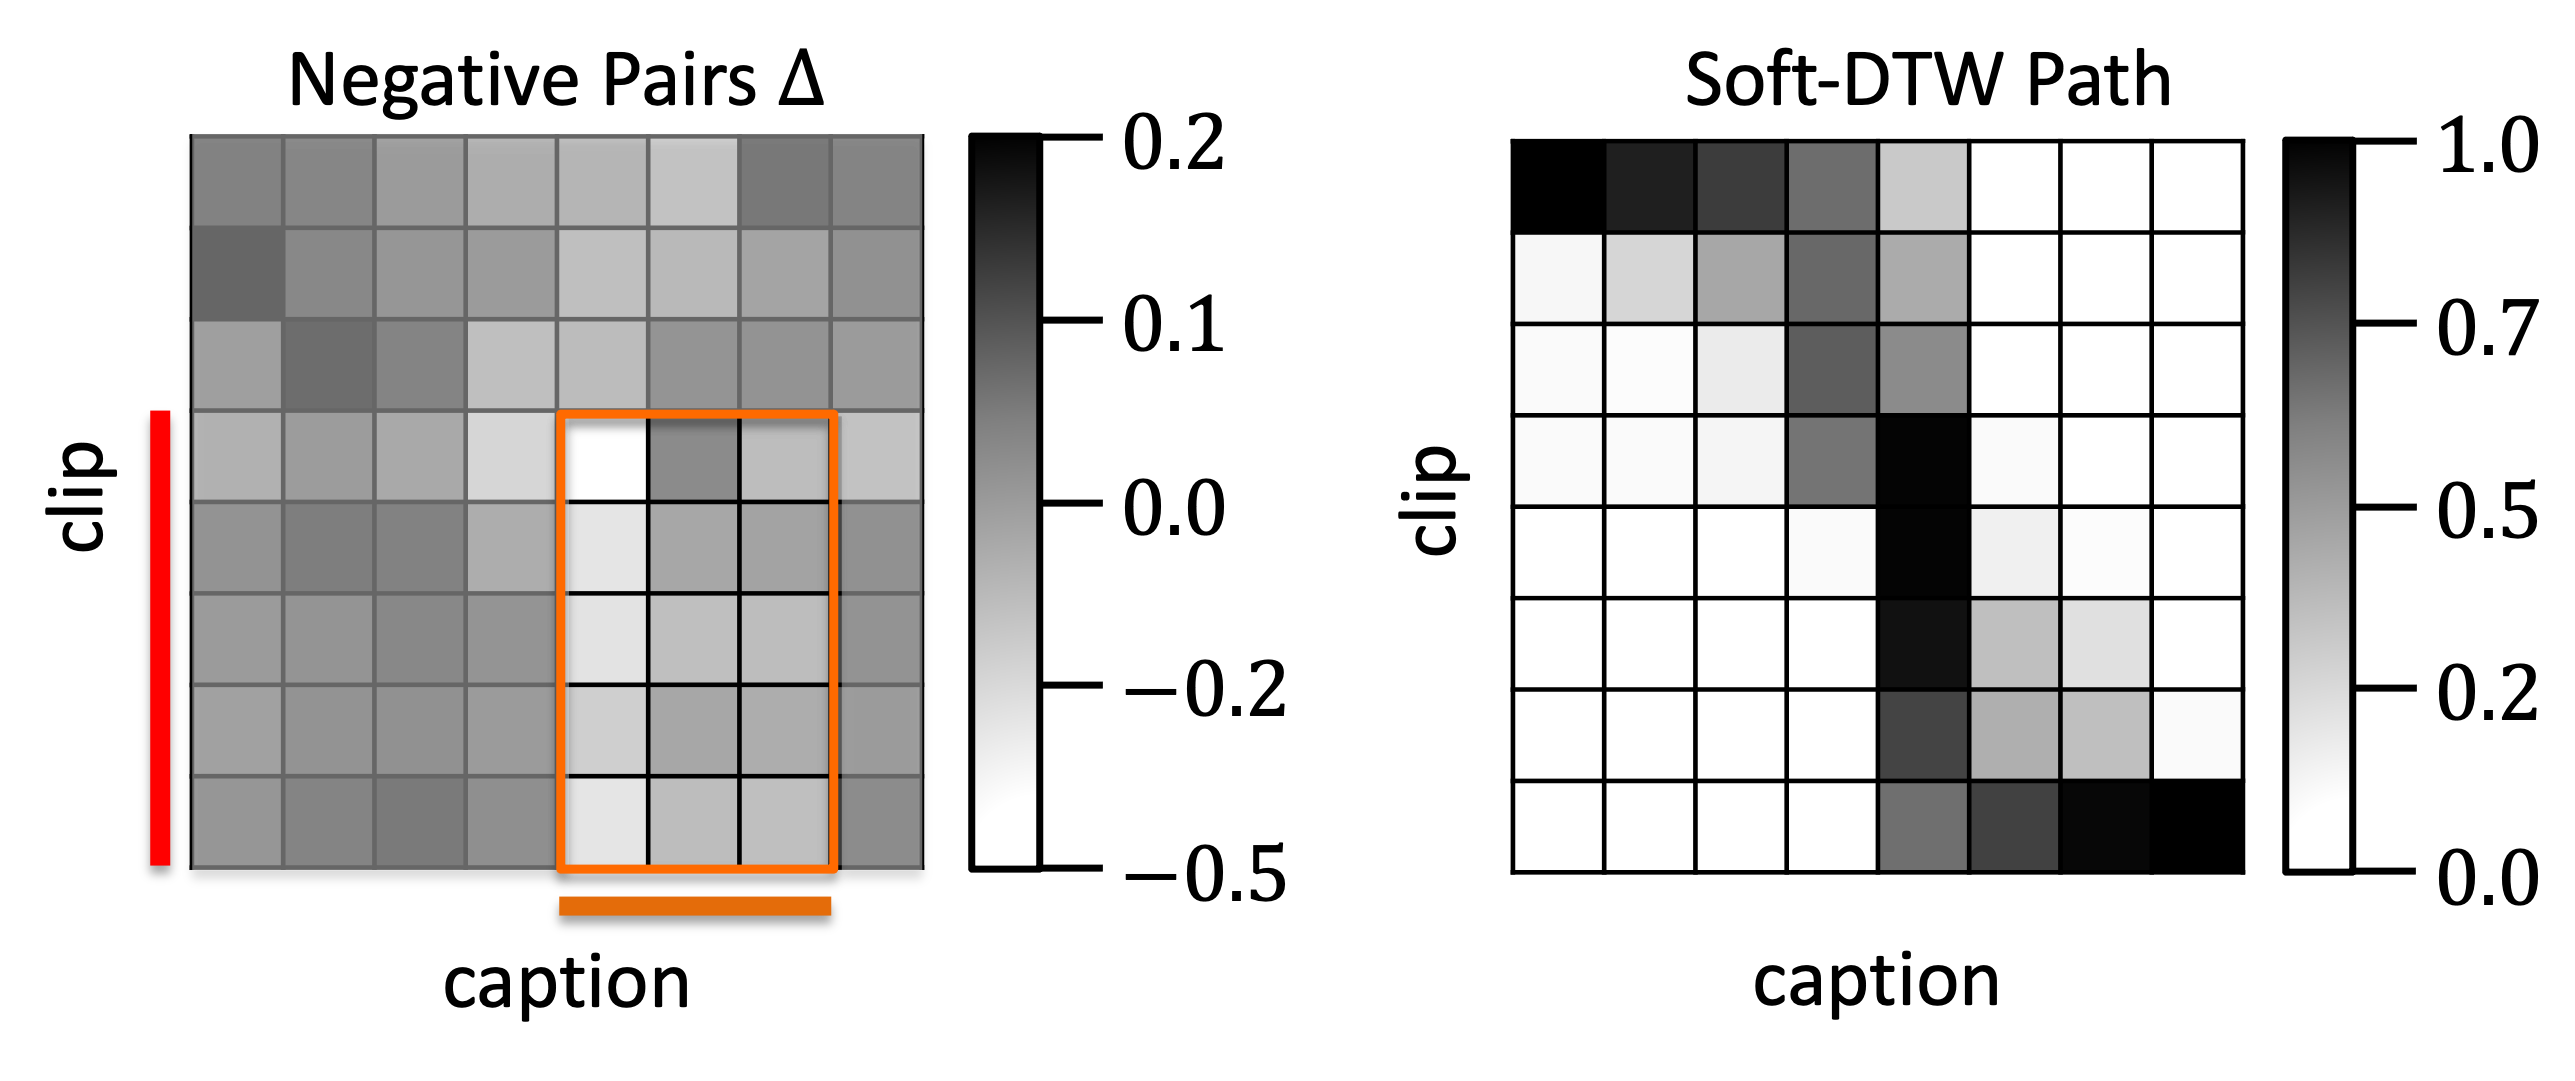}
        \caption{Negative Pairs.}
        \label{fig:negative}
    \end{subfigure}
    \caption{\textbf{Soft-DTW Path of Positive Pairs and Negative Pairs.} 
    The red box and blue box of (a) are the aligned pairs between positive clip-caption pairs.
    The orange box of (b) is the aligned pairs between negative clip-caption pairs.
    }
    \label{fig:positive_negative}
\end{figure}
