# Supplementary material for: Video-Text Representation Learning via Differentiable Weak Temporal Alignment
Source: arXiv:2203.16784 source file (2022-03-31)
Supplement: Supplementary file 4 [file supple_path.tex]

\begin{figure}
    \centering
    \begin{subfigure}[b]{0.31\textwidth}  
        \centering 
        \includegraphics[width=\textwidth]{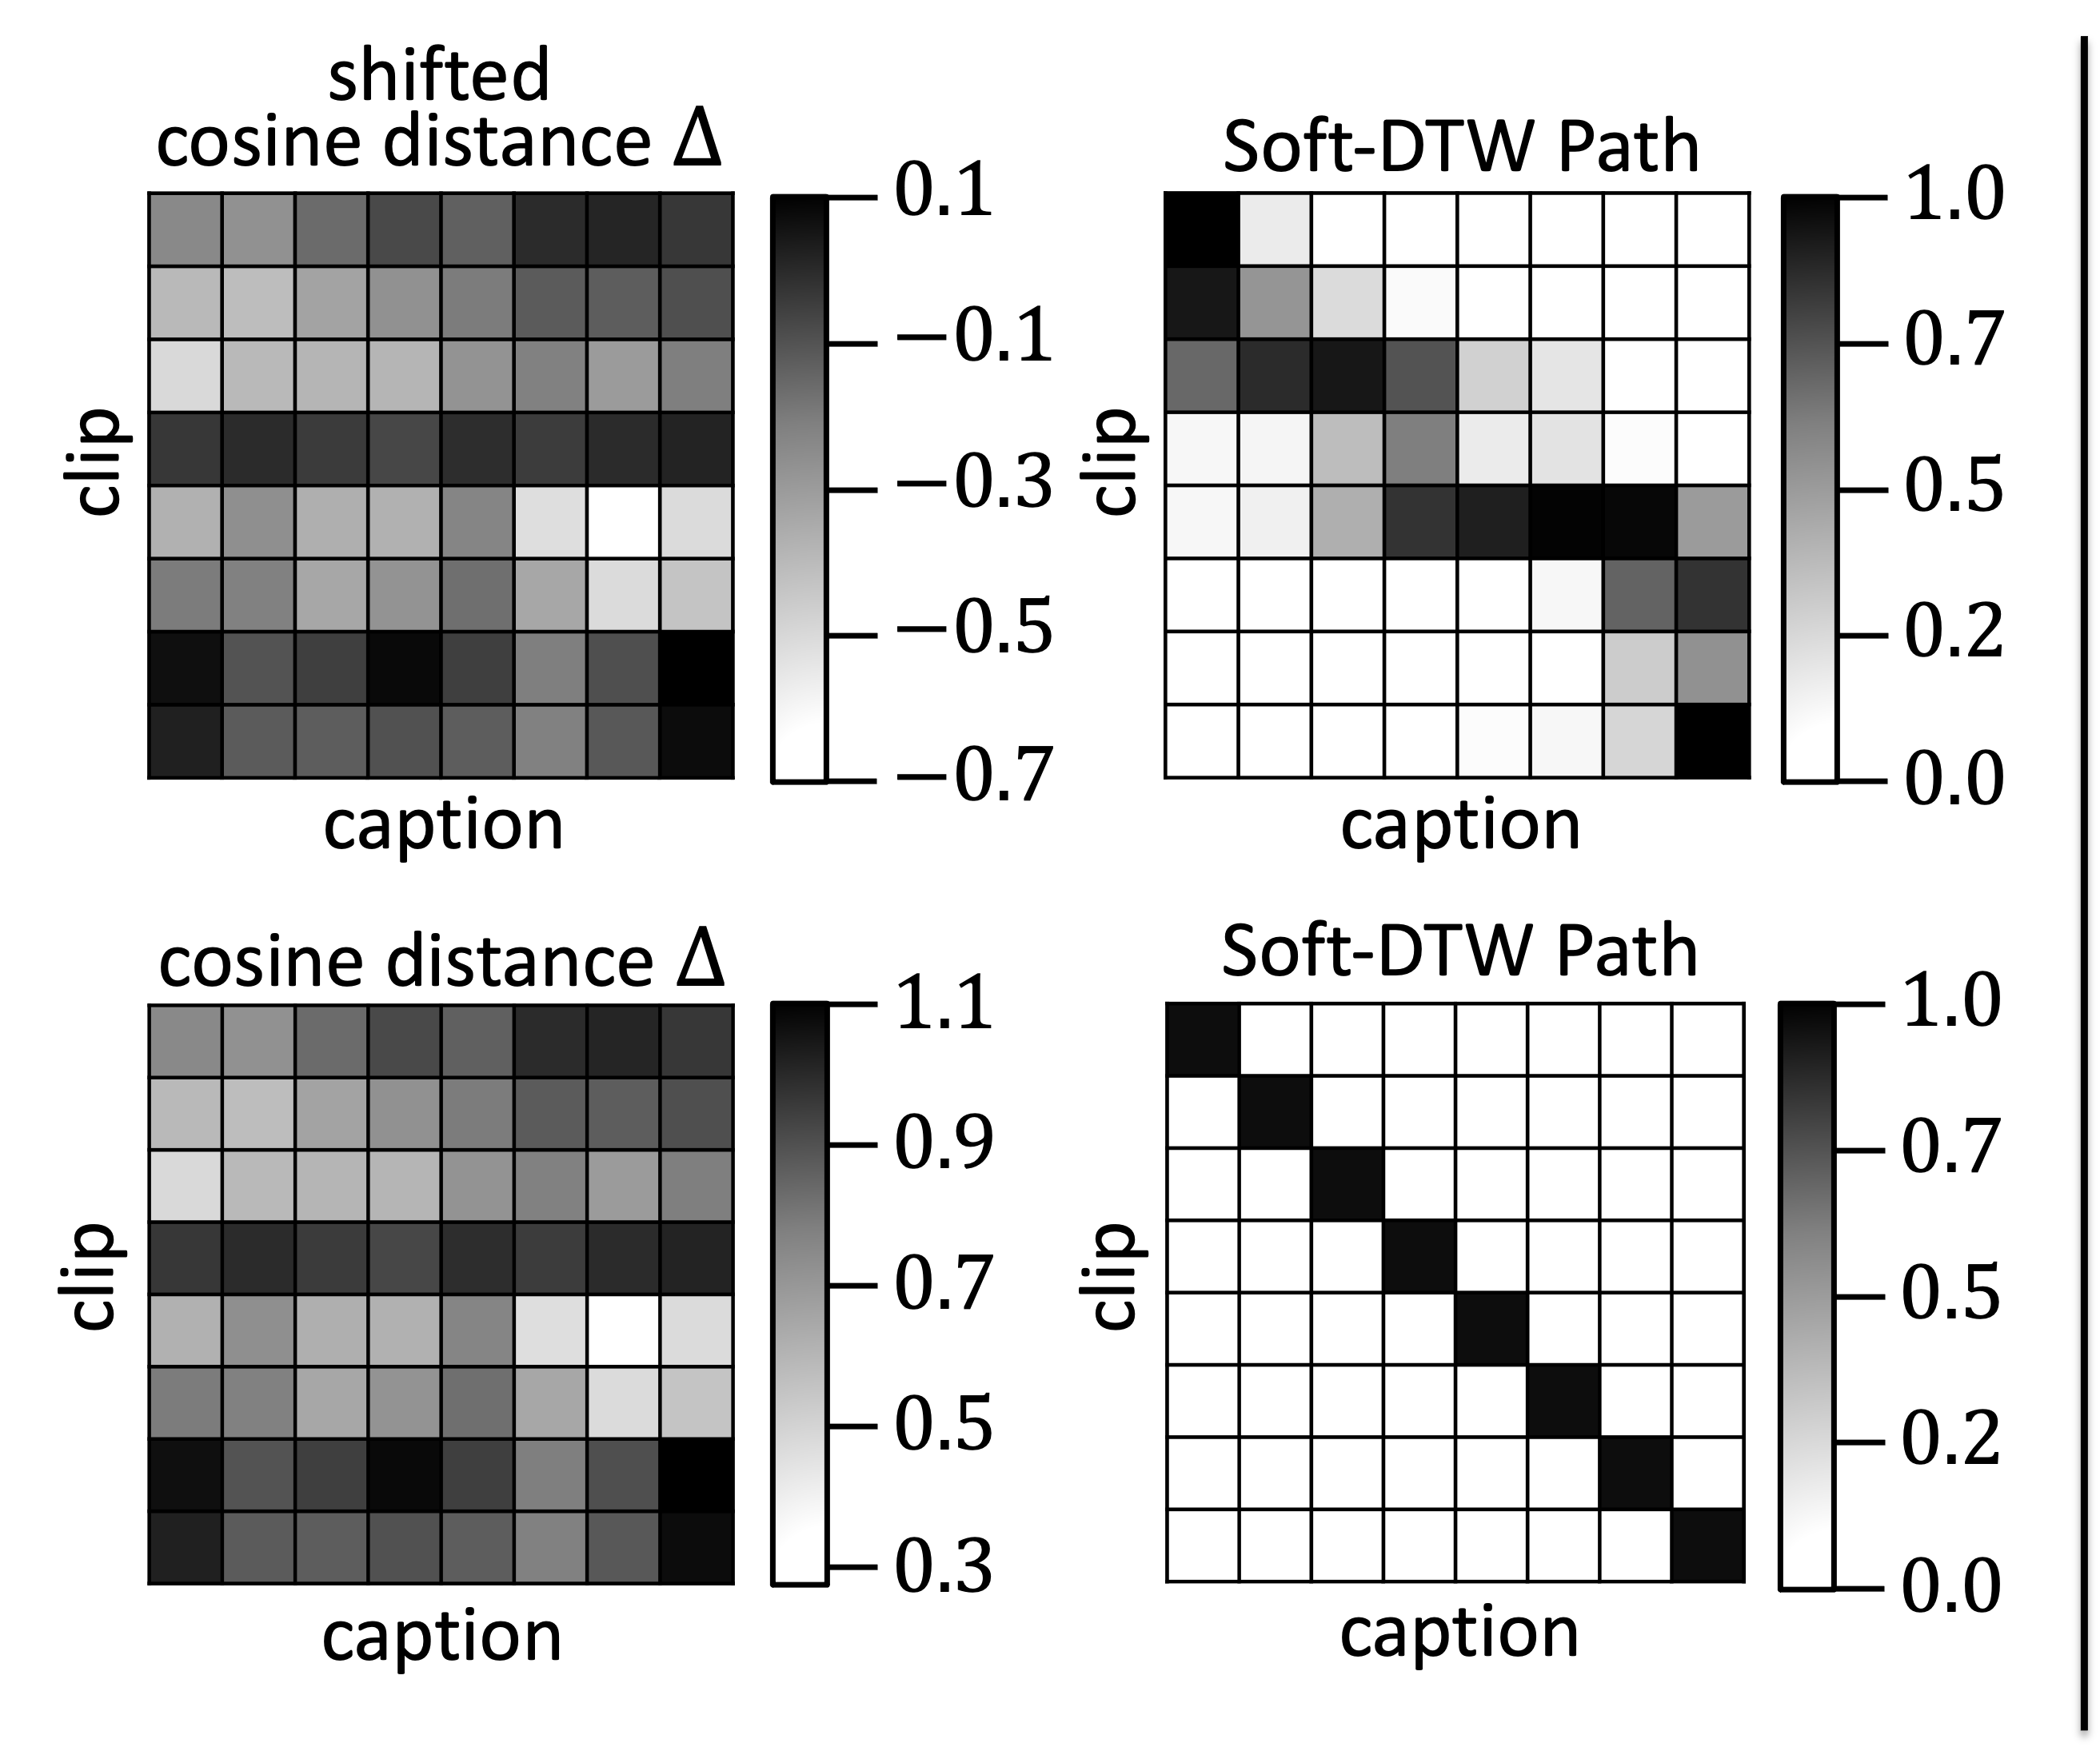}
        \caption{Cosine Distance.}
        \label{fig:cosine}
    \end{subfigure}
    \begin{subfigure}[b]{0.16\textwidth}   
        \centering 
        \includegraphics[width=\textwidth]{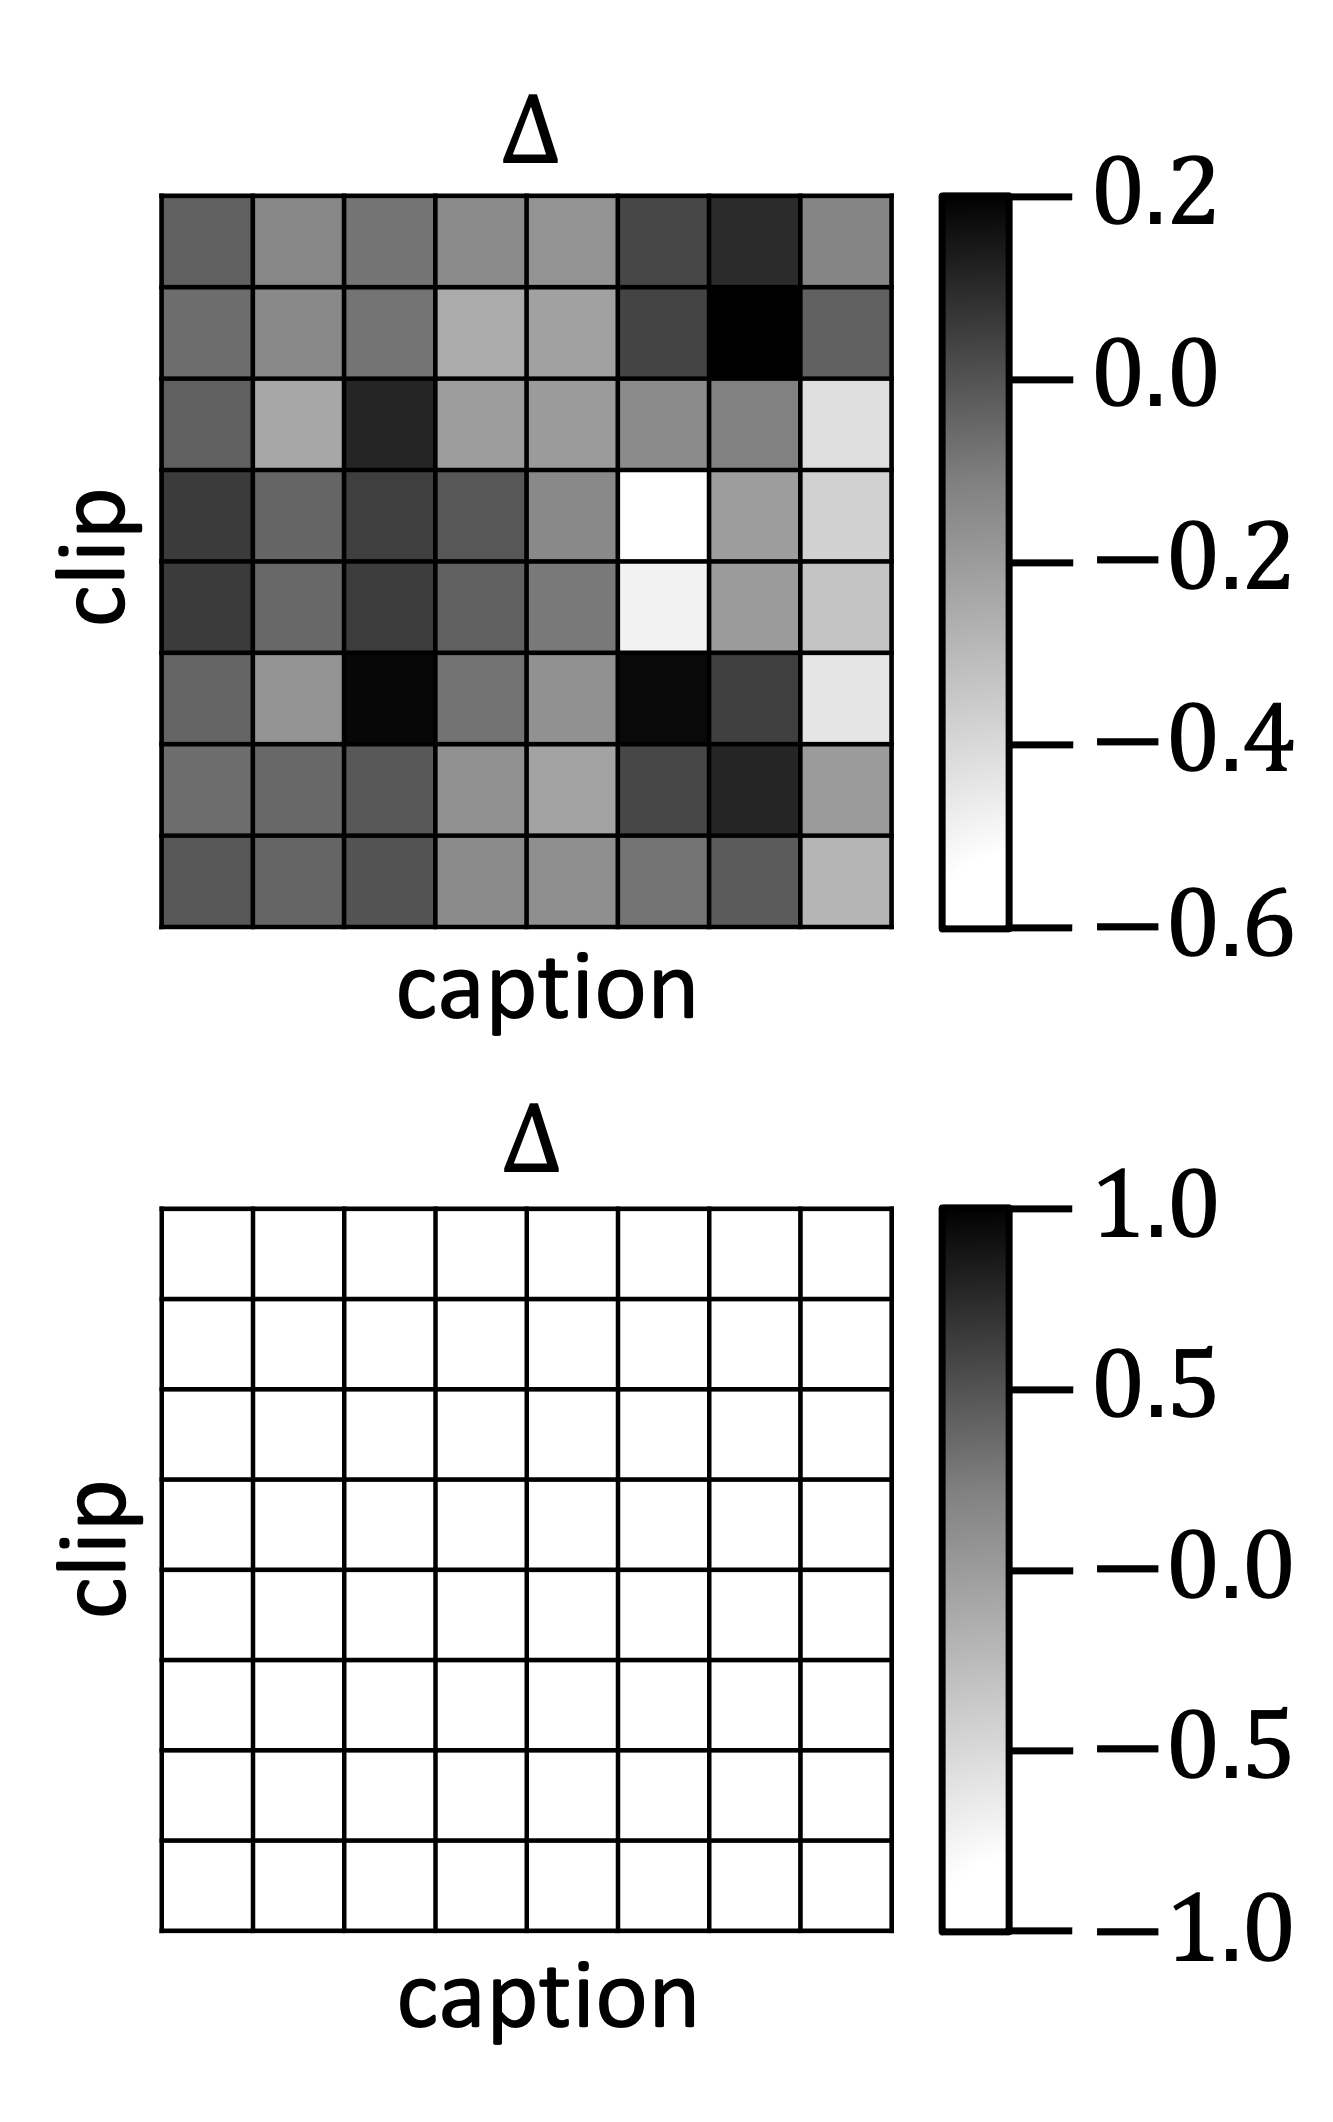}
        \caption{Feature Collapsing.}
        \label{fig:collapsing}
    \end{subfigure}
    \caption{\textbf{Results of Shifted Cosine Distance and Feature Collapsing.} 
    $\Delta$ is a pairwise distance matrix. The Soft-DTW path matrix is the gradient matrices $M$ defined in Section 4.1 of the main paper.
    }
\end{figure}
